# Supplementary material for: Gaia Data Release 1: Catalogue validation
Source: arXiv:1701.00292 source file (2017-01-01)
Supplement: Supplementary file 1 [file appendix-models.tex]

\section{Description of the models} \label{app:models}

\paragraph{Description of the models.}\label{ssec:modeldesc}
To exercise several validation tests, we benefited from the simulations
done in the frame of the Gaia DPAC, the Coordination Unit 2 being in
charge of producing theses simulations. Namely, we used the
Gaia Universe Model Snapshot \citep[GUMS, ][]{2012A&A...543A.100R} and 
the Gaia Object Generator~\citep[GOG, ][]{2014A&A...566A.119L} catalogue, which is the GUMS catalogue 
to which estimated Gaia errors have been added. In GOG version 18 (GOG18) used here, the error models have been updated, in phase with the mission Science Performance estimations\footnote{http://www.cosmos.esa.int/web/gaia/science-performance}.
The Besan\c{c}on Galactic Model (BGM)~\citep{bgm} simulates physical and dynamical properties of stars 
in the Milky May in a self-consistent manner. In addition, it includes phenomenological models 
for extinction. The model generates fake stars and predict
their properties. But these sources do not correspond to real stars in the sky. Therefore, only 
statistical properties of sources in a region or the whole sky can be compared with 
observed catalogues. All the validation tests in WP943 are consequently based 
on comparisons of statistics of physical quantities. Several mock catalogues have been generated by using 
various versions of BGM. For the comparison to whole sky up to magnitude 20, we use the GUMS or the GOG catalogue. For the comparison to TGAS data, we use the BMGBGT~\citep{2014A&A...564A.102C} catalogue, version BMGBGT-04-08~\citep{2014A&A...564A.102C} which is better adapted 
for stars with G magnitude in 9-11.5 interval and astrometric resolution of TGAS. 

In order to validate the tests and the model before Gaia data are available, we compared our specific simulation of TGAS with 
semi-empirical simulated catalogues which contains the Tycho catalogue 
with estimations of the parallaxes based on photometric distances. For the validation of the model up to magnitude 20, we compared model sky densities to SDSS and 2MASS catalogues \citep{2012A&A...538A.106R,2014A&A...569A..13R} in wide areas of the sky, which allow to establish a level of accuracy in stellar density at the level of 10\% on most of the sky and 30\% in the Galactic place (due to uncertainty on the extinction model).

\paragraph{Method.} \label{sec:method943}

Model-based validation tests share the same methodology for calculation of statistical properties and 
their comparison. The specification of tests and their implementation are described in the internal Gaia documentation.
Here we summarize definition and methodology for their calculation. Tested quantities include: 
Distribution of properties such as number, magnitudes, colours, proper motions and their moments, 
and parallax in the bins of sky, their histograms, and relation between various quantities as 
2D-histograms. They are separately calculated for data and model, and compared.

The sky is divided into equal area bins using HealPix algorithm with respect to 
galactic coordinates.

The validation code is designed such that in each test it is possible to have separate 
criteria in different latitude intervals. In this way one can minimize the uncertainty of 
validation tests due to imprecision of the model itself, as well as to study the accuracy of Gaia that might be latitude dependent. For the time being, latitude bins have been fixed to $b<-70$\deg, $-70<b<20$, $-20<b<20$, $20<b<70$, $b>70$\deg. Magnitude bins are from 9 to 11.5 by step of 0.5 magnitude for TGAS, and from 12 to 20 by bins of 1 magnitude step for the deep catalogue.

For testing sky densities, we compare in each healpixel and each magnitude range the number of stars observed by Gaia and simulated by the model. We examine the relative density and compare with a threshold and with the Poisson noise. The pixel is flagged if the relative density is larger than both of these values. The tests fail only if a larger number of healpixels are flagged as bad (typically 30\%), in order to avoid some small areas containing clusters, HII regions, or under-densities not reproduced in the model.

For testing astrometric parameter distributions, we compare the mean and standard deviations of the proper motions (on both axes) and of the parallaxes in latitude regions and in magnitude bins. The bins are flagged bad if the mean or the standard deviation of this parameter deviates more than the assumed threshold. The thresholds are established from the comparison between the model simulations performed specifically for this purpose \citep{2014A&A...564A.102C} with a Gaia simulated catalogue, ensuring that the tests passed for this comparison. Histograms of physical quantities used in the validation tests, calculated separately in magnitude and latitude intervals, determine their distribution and dispersion. 

The two main subsamples of {\GDR1} (TGAS and main GDR1) have been considered separately during the validation with models. We have done three sets of simulations, two for validating TGAS, one for validating star counts in GDR1. For TGAS models are used to estimate whether the parallax and proper motions distributions looked reasonable and do not suffer from strange systematics or random errors with regards to the magnitude of the stars and with position on the sky. For the whole {\GDR1}, models are used to estimate whether the sky density as a function of magnitude compares well with our expectations, considering the present knowledge about the Galactic stellar densities. Since in the present release there is no colour informations, differences between models and data are not always easy to understand. However, it is still useful to estimate the completeness of the catalogue.
